# Supplementary material for: Randomized Sharpness-Aware Training for Boosting Computational Efficiency in Deep Learning
Source: arXiv:2203.09962 source file (2023-04-10)
Supplement: Supplementary file 1 [file 5043_appendix.pdf]

# SS-SAM : Stochastic Scheduled Sharpness-Aware Minimization for Efficiently Training Deep Neural Networks

Anonymous ECCV submission

Paper ID 5043

## Appendix

### A Experiment Results when using Cutout Regularization

In addition to the basic data augmentation strategy used in the previous section, we would also investigate the effect when using the Cutout Regularization [1]. Here, the training hyperparameters are the same as them used in the previous sections.

The tables below show the final results, where trainings are scheduled by constant scheduling functions (Table 1), the first group of piecewise scheduling functions (Table 2) and the first group of linear scheduling functions (Table 3) and trigonometric scheduling functions (Table 4), respectively. We could see that when implementing the Cutout regularization, with proper scheduling functions, the computational cost could be reduced, while models could acquire comparable or even better generalization with the SAM training scheme.

**Table 1.** Testing error rate of WideResNet28-10 models on Cifar10 and Cifar100 datasets with Cutout regularization when training with constant scheduling functions.

|             | Cifar10           |                     |                | Cifar100           |                     |                |
|-------------|-------------------|---------------------|----------------|--------------------|---------------------|----------------|
| $a_c$       | Error[%]          | Time[m]             | $\hat{\eta}_c$ | Error[%]           | Time[m]             | $\hat{\eta}_c$ |
| SGD         | $2.81_{\pm 0.07}$ | $57.33_{\pm 0.71}$  | 1.0            | $16.91_{\pm 0.10}$ | $57.46_{\pm 0.77}$  | 1.0            |
| SAM         | $2.43_{\pm 0.13}$ | $105.17_{\pm 0.94}$ | 2.0            | $14.87_{\pm 0.16}$ | $103.14_{\pm 1.12}$ | 2.0            |
| $a_c = 0.1$ | $2.67_{\pm 0.05}$ | $61.82_{\pm 0.17}$  | 1.1            | $16.14_{\pm 0.18}$ | $62.46_{\pm 0.85}$  | 1.1            |
| $a_c = 0.2$ | $2.53_{\pm 0.06}$ | $67.52_{\pm 1.12}$  | 1.2            | $15.97_{\pm 0.16}$ | $67.85_{\pm 0.96}$  | 1.2            |
| $a_c = 0.3$ | $2.46_{\pm 0.06}$ | $72.33_{\pm 1.23}$  | 1.3            | $15.56_{\pm 0.14}$ | $72.29_{\pm 0.99}$  | 1.3            |
| $a_c = 0.4$ | $2.40_{\pm 0.06}$ | $76.31_{\pm 1.31}$  | 1.4            | $15.17_{\pm 0.22}$ | $76.04_{\pm 1.04}$  | 1.4            |
| $a_c = 0.5$ | $2.32_{\pm 0.06}$ | $80.81_{\pm 0.96}$  | 1.5            | $15.10_{\pm 0.11}$ | $80.37_{\pm 0.78}$  | 1.5            |
| $a_c = 0.6$ | $2.31_{\pm 0.07}$ | $85.60_{\pm 1.09}$  | 1.6            | $14.96_{\pm 0.08}$ | $84.98_{\pm 1.06}$  | 1.6            |
| $a_c = 0.7$ | $2.25_{\pm 0.08}$ | $89.66_{\pm 1.19}$  | 1.7            | $14.94_{\pm 0.09}$ | $89.84_{\pm 1.53}$  | 1.7            |
| $a_c = 0.8$ | $2.23_{\pm 0.03}$ | $95.05_{\pm 1.10}$  | 1.8            | $14.81_{\pm 0.09}$ | $94.42_{\pm 1.35}$  | 1.8            |
| $a_c = 0.9$ | $2.31_{\pm 0.06}$ | $98.18_{\pm 0.20}$  | 1.9            | $14.71_{\pm 0.03}$ | $97.79_{\pm 1.01}$  | 1.9            |

**Table 2.** Testing error rate of WideResNet28-10 models on Cifar10 and Cifar100 datasets with Cutout regularization when training with the first group of piecewise scheduling functions.

|             | Cifar10           |                     |                | Cifar100           |                     |                |
|-------------|-------------------|---------------------|----------------|--------------------|---------------------|----------------|
| $b_p$       | Error[%]          | Time[m]             | $\hat{\eta}_p$ | Error[%]           | Time[m]             | $\hat{\eta}_p$ |
| SGD         | $2.81_{\pm 0.07}$ | $57.33_{\pm 0.71}$  | 1.0            | $16.91_{\pm 0.10}$ | $57.46_{\pm 0.77}$  | 1.0            |
| SAM         | $2.43_{\pm 0.13}$ | $105.17_{\pm 0.94}$ | 2.0            | $14.87_{\pm 0.16}$ | $103.14_{\pm 1.12}$ | 2.0            |
| $b_p = 0.1$ | $2.19_{\pm 0.05}$ | $101.47_{\pm 1.54}$ | 1.9            | $14.75_{\pm 0.24}$ | $100.44_{\pm 1.47}$ | 1.9            |
| $b_p = 0.2$ | $2.30_{\pm 0.05}$ | $95.70_{\pm 1.39}$  | 1.8            | $14.84_{\pm 0.09}$ | $94.89_{\pm 0.70}$  | 1.8            |
| $b_p = 0.3$ | $2.34_{\pm 0.03}$ | $90.84_{\pm 1.20}$  | 1.7            | $14.99_{\pm 0.26}$ | $90.27_{\pm 0.51}$  | 1.7            |
| $b_p = 0.4$ | $2.34_{\pm 0.02}$ | $85.50_{\pm 0.18}$  | 1.6            | $14.98_{\pm 0.28}$ | $86.82_{\pm 1.19}$  | 1.6            |
| $b_p = 0.5$ | $2.46_{\pm 0.02}$ | $81.46_{\pm 0.81}$  | 1.5            | $15.24_{\pm 0.22}$ | $81.55_{\pm 1.20}$  | 1.5            |
| $b_p = 0.6$ | $2.44_{\pm 0.04}$ | $77.59_{\pm 1.02}$  | 1.4            | $15.24_{\pm 0.35}$ | $76.74_{\pm 0.62}$  | 1.4            |
| $b_p = 0.7$ | $2.47_{\pm 0.05}$ | $72.27_{\pm 0.61}$  | 1.3            | $15.38_{\pm 0.33}$ | $71.83_{\pm 0.04}$  | 1.3            |
| $b_p = 0.8$ | $2.51_{\pm 0.07}$ | $67.80_{\pm 0.64}$  | 1.2            | $15.37_{\pm 0.18}$ | $67.82_{\pm 0.71}$  | 1.2            |
| $b_p = 0.9$ | $2.69_{\pm 0.04}$ | $64.08_{\pm 0.87}$  | 1.1            | $15.70_{\pm 0.21}$ | $63.77_{\pm 0.82}$  | 1.1            |

**Table 3.** Testing error rate of WideResNet28-10 models on Cifar10 and Cifar100 datasets with Cutout regularization when training with the first group of linear scheduling functions.

|                        | Cifar10           |                     |                | Cifar100           |                     |                |
|------------------------|-------------------|---------------------|----------------|--------------------|---------------------|----------------|
| $p(\frac{T}{2})$       | Error[%]          | Time[m]             | $\hat{\eta}_p$ | Error[%]           | Time[m]             | $\hat{\eta}_p$ |
| SGD                    | $2.81_{\pm 0.07}$ | $57.33_{\pm 0.71}$  | 1.0            | $16.91_{\pm 0.10}$ | $57.46_{\pm 0.77}$  | 1.0            |
| SAM                    | $2.43_{\pm 0.13}$ | $105.17_{\pm 0.94}$ | 2.0            | $14.87_{\pm 0.16}$ | $103.14_{\pm 1.12}$ | 2.0            |
| $p(\frac{T}{2}) = 0.1$ | $2.63_{\pm 0.02}$ | $63.08_{\pm 0.15}$  | 1.1            | $15.83_{\pm 0.27}$ | $62.97_{\pm 0.46}$  | 1.1            |
| $p(\frac{T}{2}) = 0.2$ | $2.58_{\pm 0.06}$ | $67.32_{\pm 0.09}$  | 1.2            | $15.67_{\pm 0.16}$ | $67.53_{\pm 0.18}$  | 1.2            |
| $p(\frac{T}{2}) = 0.3$ | $2.45_{\pm 0.05}$ | $72.11_{\pm 0.01}$  | 1.3            | $15.33_{\pm 0.17}$ | $72.09_{\pm 0.09}$  | 1.3            |
| $p(\frac{T}{2}) = 0.4$ | $2.37_{\pm 0.07}$ | $77.01_{\pm 0.87}$  | 1.4            | $15.30_{\pm 0.19}$ | $76.91_{\pm 0.38}$  | 1.4            |
| $p(\frac{T}{2}) = 0.5$ | $2.38_{\pm 0.02}$ | $80.73_{\pm 0.11}$  | 1.5            | $15.33_{\pm 0.11}$ | $81.19_{\pm 0.69}$  | 1.5            |
| $p(\frac{T}{2}) = 0.6$ | $2.27_{\pm 0.10}$ | $86.65_{\pm 1.41}$  | 1.4            | $14.97_{\pm 0.02}$ | $86.93_{\pm 0.42}$  | 1.4            |
| $p(\frac{T}{2}) = 0.7$ | $2.25_{\pm 0.03}$ | $91.20_{\pm 1.62}$  | 1.7            | $14.95_{\pm 0.23}$ | $91.78_{\pm 0.32}$  | 1.7            |
| $p(\frac{T}{2}) = 0.8$ | $2.22_{\pm 0.03}$ | $94.25_{\pm 0.12}$  | 1.8            | $14.68_{\pm 0.14}$ | $94.29_{\pm 0.53}$  | 1.8            |
| $p(\frac{T}{2}) = 0.9$ | $2.23_{\pm 0.10}$ | $99.69_{\pm 0.59}$  | 1.9            | $14.79_{\pm 0.04}$ | $100.57_{\pm 0.72}$ | 1.9            |

**Table 4.** Testing error rate of WideResNet28-10 models on Cifar10 and Cifar100 datasets with Cutout regularization when training with two trigonometric scheduling functions.

|                  | Cifar10           |                     |                | Cifar100           |                     |                |
|------------------|-------------------|---------------------|----------------|--------------------|---------------------|----------------|
| $p(\frac{T}{2})$ | Error[%]          | Time[m]             | $\hat{\eta}_p$ | Error[%]           | Time[m]             | $\hat{\eta}_p$ |
| SGD              | $2.81_{\pm 0.07}$ | $57.33_{\pm 0.71}$  | 1.0            | $16.91_{\pm 0.10}$ | $57.46_{\pm 0.77}$  | 1.0            |
| SAM              | $2.43_{\pm 0.13}$ | $105.17_{\pm 0.94}$ | 2.0            | $14.87_{\pm 0.16}$ | $103.14_{\pm 1.12}$ | 2.0            |
| $p_{\cos 2}(t)$  | $2.35_{\pm 0.03}$ | $81.49_{\pm 0.39}$  | 1.5            | $15.02_{\pm 0.19}$ | $80.83_{\pm 0.55}$  | 1.5            |
| $p_{\sin 1}(t)$  | $2.27_{\pm 0.04}$ | $80.39_{\pm 1.53}$  | 1.5            | $14.85_{\pm 0.17}$ | $81.15_{\pm 0.53}$  | 1.5            |

## B Other Experiment Results for VGG Models

Other than WideResNet28-10, we would also investigate another model architecture, namely the VGG16 [2] with batch normalization. From the previous results, we could see that the constant scheduling functions would already provide representative results. So here we would only investigate the results when trained with constant scheduling functions. Table 5 shows the results, where the running time is reported on one A100 Nvidia GPU. We could see in the table that SS-SAM again could boost the computational efficiency and in the meantime acquire better model generalization compared to that trained using the SAM scheme.

**Table 5.** Testing error rate of VGG16-BN models on Cifar10 and Cifar100 datasets when training with constant scheduling functions.

|             | Cifar10           |                    |                | Cifar100           |                    |                |
|-------------|-------------------|--------------------|----------------|--------------------|--------------------|----------------|
| $a_c$       | Error[%]          | Time[m]            | $\hat{\eta}_c$ | Error[%]           | Time[m]            | $\hat{\eta}_c$ |
| SGD         | $5.74_{\pm 0.09}$ | $12.18_{\pm 0.21}$ | 1.0            | $25.22_{\pm 0.31}$ | $12.07_{\pm 0.37}$ | 1.0            |
| SAM         | $5.24_{\pm 0.08}$ | $20.41_{\pm 0.57}$ | 2.0            | $24.23_{\pm 0.29}$ | $20.33_{\pm 0.68}$ | 2.0            |
| $a_c = 0.1$ | $5.49_{\pm 0.08}$ | $13.04_{\pm 0.21}$ | 1.1            | $24.90_{\pm 0.21}$ | $12.93_{\pm 0.19}$ | 1.1            |
| $a_c = 0.2$ | $5.25_{\pm 0.07}$ | $13.66_{\pm 0.14}$ | 1.2            | $24.83_{\pm 0.17}$ | $13.77_{\pm 0.39}$ | 1.2            |
| $a_c = 0.3$ | $5.19_{\pm 0.07}$ | $14.40_{\pm 0.30}$ | 1.3            | $24.08_{\pm 0.12}$ | $14.53_{\pm 0.17}$ | 1.3            |
| $a_c = 0.4$ | $5.29_{\pm 0.03}$ | $15.25_{\pm 0.42}$ | 1.4            | $24.23_{\pm 0.20}$ | $15.41_{\pm 0.23}$ | 1.4            |
| $a_c = 0.5$ | $5.05_{\pm 0.05}$ | $16.11_{\pm 0.37}$ | 1.5            | $23.83_{\pm 0.17}$ | $16.18_{\pm 0.32}$ | 1.5            |
| $a_c = 0.6$ | $5.15_{\pm 0.02}$ | $17.14_{\pm 0.52}$ | 1.6            | $24.12_{\pm 0.11}$ | $17.16_{\pm 0.28}$ | 1.6            |
| $a_c = 0.7$ | $4.97_{\pm 0.04}$ | $17.72_{\pm 0.22}$ | 1.7            | $23.86_{\pm 0.18}$ | $18.03_{\pm 0.47}$ | 1.7            |
| $a_c = 0.8$ | $4.89_{\pm 0.05}$ | $18.56_{\pm 0.56}$ | 1.8            | $23.97_{\pm 0.14}$ | $18.72_{\pm 0.37}$ | 1.8            |
| $a_c = 0.9$ | $4.91_{\pm 0.06}$ | $19.66_{\pm 0.31}$ | 1.9            | $23.81_{\pm 0.15}$ | $19.62_{\pm 0.29}$ | 1.9            |

## C Training Details

The basic training hyperparameters are deployed as below,

**Table 6.** The basic hyperparameters for training.

|                          | Cifar10 & Cifar100 |
|--------------------------|--------------------|
| Epoch                    | 200                |
| Batch size               | 256                |
| Basic learning rate      | 0.1                |
| Learning rate schedule   | cosine             |
| Weight decay             | 0.001              |
| $\rho$ in SAM and SS-SAM | 0.1                |

## References

1. Devries, T., Taylor, G.W.: Improved regularization of convolutional neural networks with cutout. arXivPreprint **abs/1708.04552** (2017), <http://arxiv.org/abs/1708.04552>
2. Simonyan, K., Zisserman, A.: Very deep convolutional networks for large-scale image recognition. In: 3rd International Conference on Learning Representations, ICLR 2015 (2015)
